# Supplementary material for: Revising deep learning methods in parking lot occupancy detection
Source: arXiv:2306.04288 source file (2024-02-12)
Supplement: Supplementary file 1 [file patch_based_results_en_b0_cross.tex]

\centering
    \caption{F1-score for cross-evaluation of EfficientNet-B0}
    \smallskip
    \begin{tabularx}{355px}{X|X|X|X|X|X}
        \toprule
        \multicolumn{1}{l|}{} & ACMPS & ACPDS & CNRPark & PKLot & SPKL \\
        \midrule
        \multicolumn{1}{l|}{ACMPS} & \textbf{0.9991} & 0.8758 & 0.9418 & 0.8890 & 0.7982 \\
        \multicolumn{1}{l|}{ACPDS} & 0.8702 & \textbf{0.9644} & 0.9448 & 0.9559 & 0.8324 \\ 
        \multicolumn{1}{l|}{CNRPark} & - & - & - & - & - \\ 
        \multicolumn{1}{l|}{PKlot} & 0.8150 & 0.8494 & 0.9223 & \textbf{0.9987} & 0.8103 \\ 
        \multicolumn{1}{l|}{SPKL} & 0.7628 & 0.7857 & 0.9235 & 0.9216 & \textbf{0.9821} \\ 
        \bottomrule
        
    \end{tabularx}
