# Supplementary material for: Revising deep learning methods in parking lot occupancy detection
Source: arXiv:2306.04288 source file (2024-02-12)
Supplement: Supplementary file 3 [file patch_based_results_vgg_19_cross.tex]

\centering
    \caption{F1-score for cross-evaluation of VGG-19}
    \smallskip
    \begin{tabularx}{355px}{X|X|X|X|X|X}
        \toprule
        \multicolumn{1}{l|}{} & ACMPS & ACPDS & CNRPark & PKLot & SPKL \\
        \midrule
        \multicolumn{1}{l|}{ACMPS} & - & - & - & - & - \\
        \multicolumn{1}{l|}{ACPDS} & - & - & - & - & - \\ 
        \multicolumn{1}{l|}{CNRPark} & - & - & - & - & - \\ 
        \multicolumn{1}{l|}{PKlot} & - & - & - & - & - \\ 
        \multicolumn{1}{l|}{SPKL} & - & - & - & - & - \\ 
        \bottomrule
        
    \end{tabularx}
